# Supplementary material for: Infographics Wizard: Flexible Infographics Authoring and Design Exploration
Source: arXiv:2204.09904 source file (2022-05-08)
Supplement: Supplementary file 1 [file supplement.tex]

\section{Appendix A \\Infographics Dataset Annotation with Visual Groups}
\label{s:dataset}
\subsection{Source Images}
We used the study results by Lu \textit{et al.} \cite{lu2020exploring} to sample 1000 infographics belonging to each of the 12 VIF categories (as proposed in their work \cite{lu2020exploring}) and in the ratio as they appear in the original dataset (Figure 8 in \cite{lu2020exploring}). Because of our framework's design aspect, since we aimed to relate the VG designs with VIF layouts, sampling infographic images based on the VIF layout was crucial for consistency with real-world designs.  

\subsection{Experiment Setup}
We annotated the infographics using Amazon Mechanical Turk \cite{mturk}. The workers were first introduced to the concept of VGs and their individual components with some example images. The task was to segment individual VGs, the components inside the VGs (refer to Figure 3B of the paper), and annotate VGs with a bounding box in each of the infographic images. For consistency, each image was annotated by three different workers, and we chose the best annotated VGs for each image manually. An example user annotated image is shown in Figure 3C in the paper. Some example user annotations are provided in the supplementary material. 

% \begin{figure}[tb]
%     \centering
%     \includegraphics[width=\columnwidth]{figures/dataset_sample}
%     \caption{Example of segmented VGs in our infographics dataset. Each VG and their individual components are segmented by human workers. }
%     \label{fig:dataset_sample}
% \end{figure}

\subsection{Processing the Segmentation Maps}
Human-generated segmentation maps are coarse with ill-defined shapes. To generate a well-defined VG segmentation map, we employed the automated GrabCut \cite{rother2004grabcut} algorithm, similar to \cite{chen2019towards}. The human annotations were used as input to the algorithm to generate high-quality segmentation masks for VGs. This mask was then passed as input to Solaris \cite{solaris} which generated SVG paths for segmented VG designs. Finally, we added additional components to the SVG based on bounding box annotations of individual VGs, provided with the dataset by Lu \textit{et al.} \cite{lu2020exploring}.

\section{Appendix B \\ Design Component Extraction}

In this section, we discuss the process of extracting VIF, VGs and Connection designs from the infographics dataset. 

\subsection{Visual Information Flow (VIF) Extraction}
VIF is the first component of our framework (\textbf{D1}), representing the backbone layout inside an infographic. As shown in Figure 3A of the paper, VIF represents the direction of information flow following the positions of repeated VGs inside an infographic. It is represented as a series of 2D points where each point represents a VG position in two dimensions corresponding to a design area, and the number of points represents the number of VGs in that particular flow. The sequence of points represents the sequence of visual groups based on the information flow. To calculate the VIF for a given infographic, we used the algorithm discussed in \cite{lu2020exploring}. %This satisfies the design component D1 from the formative study. 

\subsection{Visual Group Design Extraction}
%We curated the VG designs from multiple sources to facilitate the infographic generation, satisfying design component D2. 
Since VG designs are the basic building block for infographic generation in our framework (\textbf{D2}), we chose multiple sources to collect VG designs to attain maximum coverage. Out of the total three sources we used, the first one is Adobe Stock \cite{adobe}, which contains SVG designs of several human-generated infographics, from which we manually separated the VG designs; the second source is our human segmented VG dataset which we curated for this work, explained in Appendix A; the third source is taken from the work by Chen \textit{et al.} \cite{chen2019towards} where we extracted VGs from timeline infographics using a Mask R-CNN \cite{he2017mask}, explained in the following text. 

These sources were carefully chosen so that we get the VG designs created directly by humans and also using automated deep learning networks. We chose the SVG format to store the VG designs because of various benefits like scaling, color, and widespread usability. Each VG is further divided into four components as shown in Figure 3B in the paper, namely: \textit{Label}, \textit{Text}, \textit{Title}, and \textit{Image}. Each VG can contain any number of these elements, and each SVG design contains separate markings for each component, which the user's content can then replace as per our design pipeline.

\subsubsection{Mask R-CNN for Initial Element Segmentation}
\label{ss:vg_maskrcnn}

\begin{figure*}[tb]
    \centering
        % $\begin{array}{cccc}
        \includegraphics[width=\textwidth]{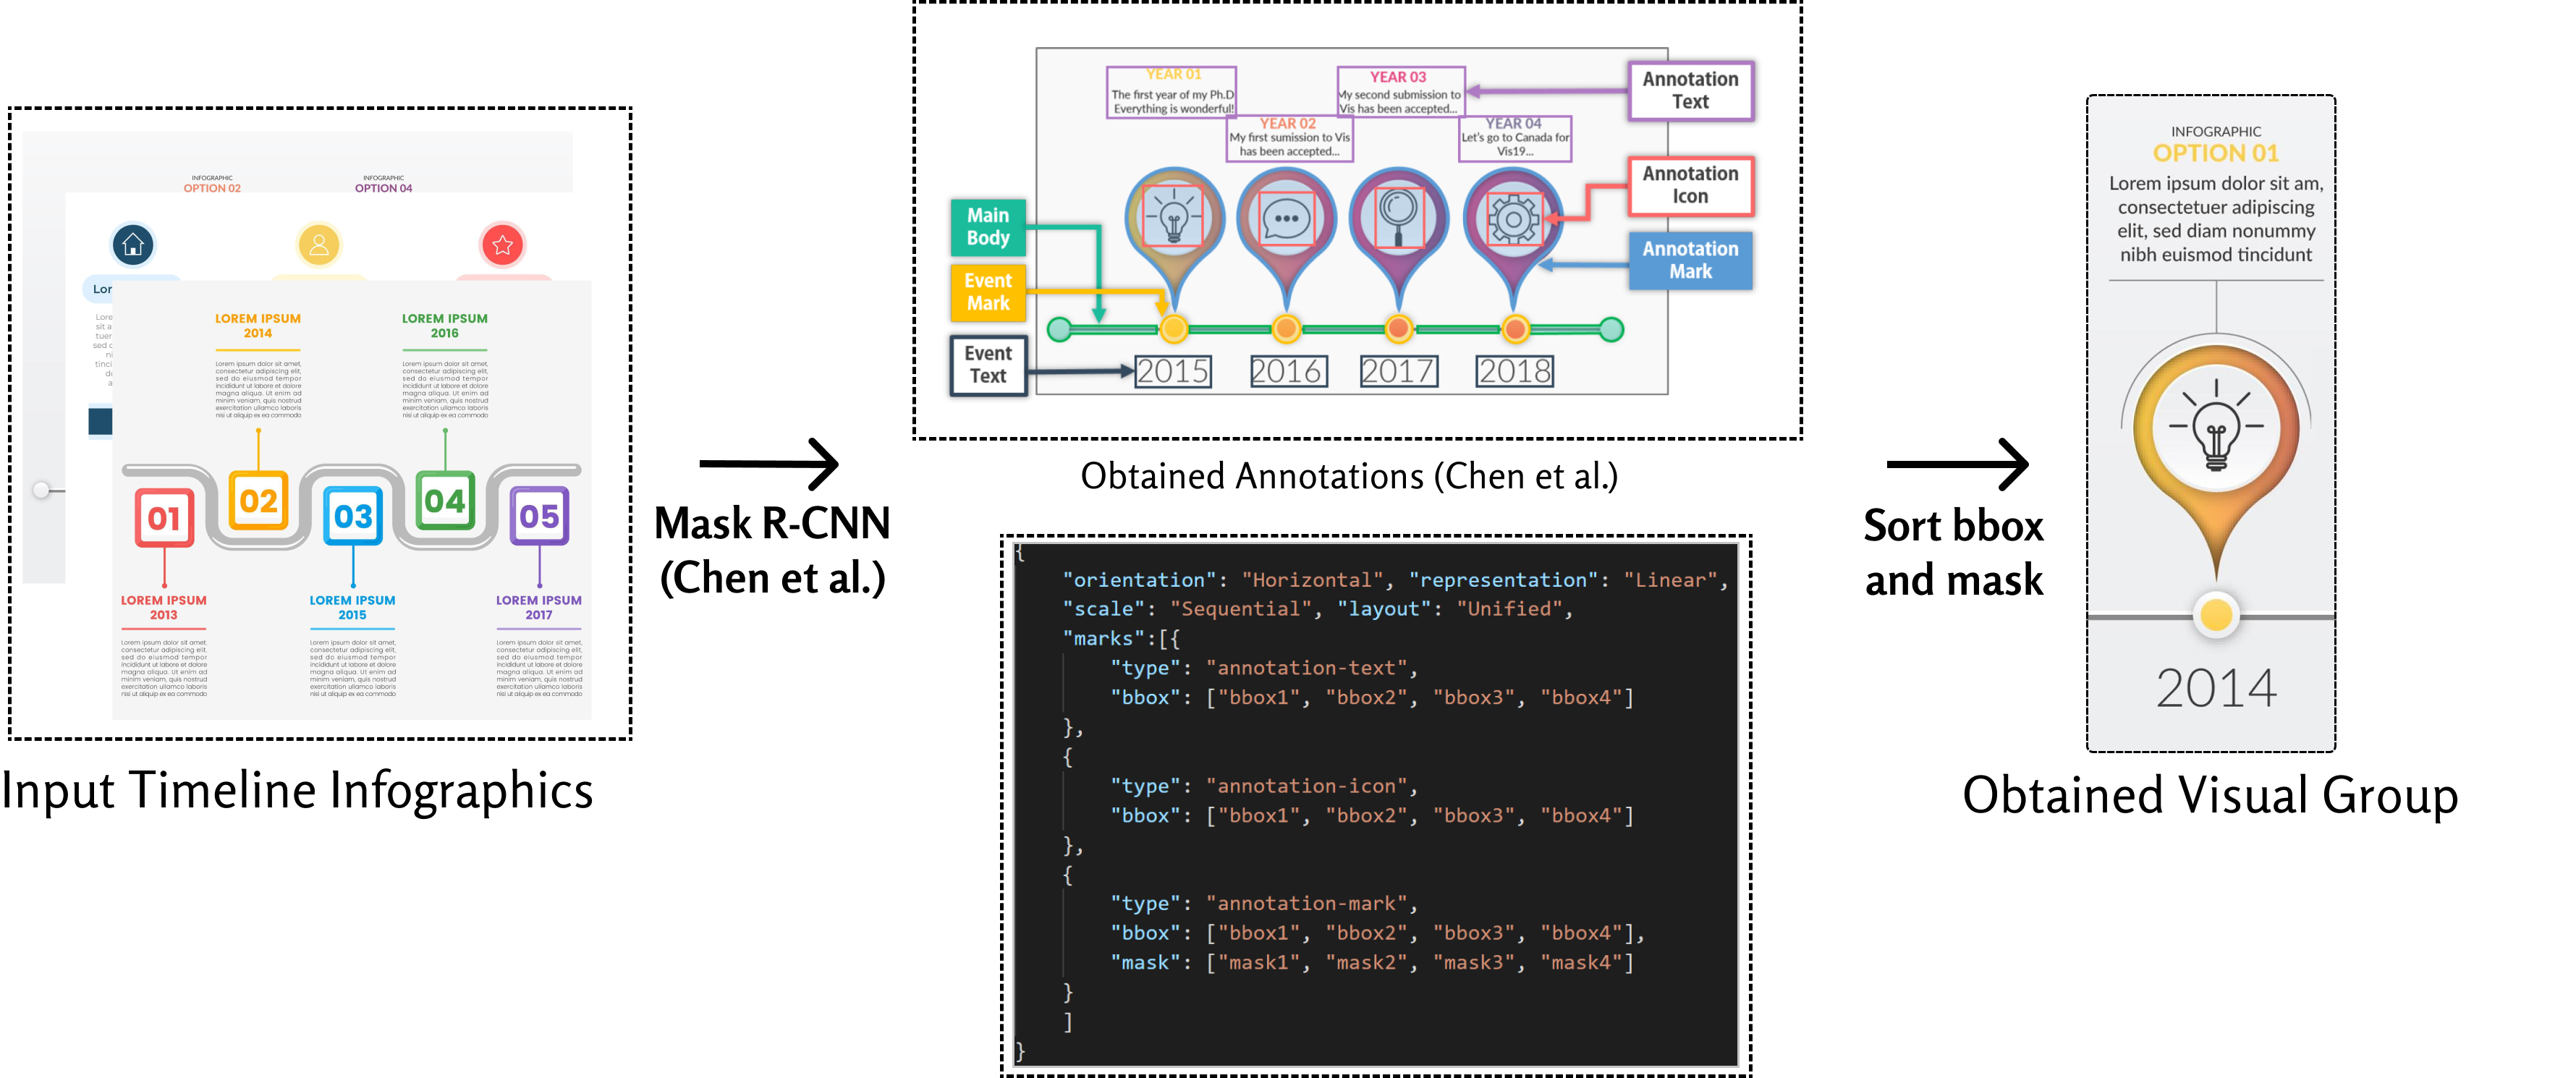}
        % \vspace{-7mm}
    \caption{Process of generating VG designs from the Mask R-CNN network. After generating the network's annotations, the bounding box and mask values are sorted in the direction perpendicular to the predicted orientation. Then the first values of every bounding box and mask are grouped to get a VG.}
    \label{fig:mask_rcnn}
\end{figure*}

In addition to the VG designs generated from the datasets available at Adobe Stock \cite{adobe}, we modified the timeline infographics work by Chen \textit{et al.} \cite{chen2019towards} to extract more VG designs. The timeline infographics dataset released with this work contains 9592 manually created timeline infographics from Timeline Storyteller \cite{brehmer2019timeline} and 1138 infographics from online sources. It includes 4689 images with manually labeled infographics components. 

We used Mask R-CNN \cite{he2017mask} with this dataset to generate the segmentation maps for the infographic components. Besides predicting the segmentation masks, a modified network predicts the local and global information about a timeline infographic image. 
The global information predicted by the network is the infographic \textit{Representation}, \textit{Scale}, \textit{Layout}, and \textit{Orientation}. For example, an infographic can have the global properties \textit{Linear}, \textit{Sequential}, \textit{Unified}, and \textit{Horizontal}, as shown in Figure \ref{fig:mask_rcnn}. Besides the global information, the network also predicts the bounding boxes for local information like \textit{Text}, \textit{Label}, \textit{Title} and \textit{Icon} along with the segmentation masks for the designs containing these elements. Figure \ref{fig:mask_rcnn} shows the network and sample annotations, respectively. The complete details of these global and local properties can be found in \cite{chen2019towards}. 

As we can see, the output of the above model provides us with the annotation labels of \textit{Text}, \textit{Icon} and \textit{Mark} and event labels of \textit{Mark} and \textit{Text} along with \textit{Main Body} labels. We can convert each of these labels to the corresponding VG elements based on the relations shown in Table \ref{tab:relations}. The entire pipeline is shown in Figure \ref{fig:mask_rcnn}.

\begin{table}[tb]
\caption{Relations of VG Elements with the Timeline Infographics prediction from Mask-RCNN}
\label{tab:relations}
\small
\begin{tabular}{
    r
    *{2}{c}
    *{5}{r}
}
\toprule
  \textbf{Timeline Component} & \textbf{Visual Group Component} \\
  \midrule
  Annotation Text & Text and Title \\
  %\midrule
  Annotation Icon & Icon \\
  %\midrule
  Annotation Mark & Visual Group Design \\
  %\midrule
  Event Mark & Connecting Point \\
  %\midrule
  Event Text & Label \\
 \bottomrule
\end{tabular}
\end{table}

\subsubsection{Visual Group SVG Generation}
Creating reusable VG designs from the Mask R-CNN predictions requires binding several predicted bounding boxes based on their respective VGs. Since the Mask R-CNN output does not predict which VG a particular bounding box belongs to, we developed a simple scheme to bind the bounding boxes based on their respective VG positions. Also, since the purpose here is to get the VG design, we only created one VG component from each infographic. We assume that the design of the VGs remains consistent within the infographic, which was found to be true in all the timeline infographics from the dataset by Lu \textit{et al.}

Hence, after predicting various elements for a given infographic image, we used the \textit{Orientation} as predicted by the Mask R-CNN to generate the VG design. We assumed that VGs are spread in the direction perpendicular to the infographic orientation. For example, in Figure \ref{fig:mask_rcnn}, the VGs extend in a vertical direction when the infographic is horizontal. Using this assumption, after generating the marks from Mask R-CNN for each of the infographic design elements, we sorted every element based on the bounding box centers in the direction perpendicular to the predicted orientation. 
After, we assigned the first element of each predict mark to the same VG. 
%After the sorted results, each predicted mark's first element belongs to the same VG. 

For simplicity, to solve the purpose of extracting meaningful VG designs, we only used the infographics with \textit{Horizontal} and \textit{Vertical} orientations. Also, we confirmed the extracted VG designs by a human analyst for their correctness and discarded the incorrectly generated VGs. The final bounding boxes and masks obtained from this process were converted to the SVG-based VG designs using Solaris \cite{solaris}.

\subsection{Connection SVG Generation}
We collected connection SVG designs from adobe stock similar to the collected 200 infographics from the formative study. All connections from these images were found on the portal, which mainly were simple shapes (like arrow, line, circle, etc.) which could be modified based on certain conditions. 

\section{Appendix C \\VIF layout Recommendation}
Following up from Equation 1 from the paper, $E_{O}$ is an indicator function that is 1 if and
only if none of the VIF flow elements lie in the boundaries of the bounding box of the pivot element, and 0 otherwise. Another component of the layout scoring energy function is $E_{C}$, which calculates the score based on the coverage a VIF layout provides. More the coverage, the higher the value of $E_{C}$, as shown in Equation~\eqref{eq:em}. Here $Hull(VIF)$ means the convex hull of the points in a particular VIF layout. 
\begin{equation}
    \label{eq:em}
    E_{C} = \frac {Area\ of\ Hull(VIF)}{Area\ of\ Canvas}
\end{equation}

The last component of the layout scoring function is the uniformity in the distance of the VIF elements wrt to the center of the pivot elements. To calculate this, we first calculate the center of the bounding box of the pivot element, denoted as $P_{XC}$ and $P_{YC}$, shown in Equation~\eqref{eq:pxc} and \eqref{eq:pyc}.
\begin{equation}
    \label{eq:pxc}
    P_{XC} = P_{X} + \frac{P_{L}}{2}
\end{equation}

\begin{equation}
    \label{eq:pyc}
    P_{YC} = P_{Y} + \frac{P_{W}}{2}
\end{equation}

Then, we calculate the variance of the distance between each VIF element and the pivot center, which gives a score of uniformity in the spread of the layout, shown in Equation~\eqref{eq:eu}. Lesser the value of $E_{U}$, the better the uniformity and vice versa. $\bar{D}$ is the mean Euclidean distance between the VIF elements and the pivot center. 
\begin{equation}
    \label{eq:eu}
    E_{U} = \frac {\sum_{X_{i}, Y_{i} \in VIF} \sqrt{(X_{i}-P_{XC})^2 + (Y_{i}-P_{YC})^2} - \bar{D}}{N}
\end{equation}

\subsubsection{VG-VIF Index}
\label{ss:vg_vif}

\begin{table}[tb]
\caption{A VG-VIF index stores the information of VGs, and the corresponding VIF cluster centers \textit{CL-$X$} in which they appear. Each VIF layout is clustered into one of the total twelve classes, shown as CL-$X$.}
\label{tab:vg-vif}
\small
\begin{tabular}{
    r
    *{2}{c}
    *{5}{r}
}
\toprule
  \textbf{Visual Group ID} & \textbf{VIF Layout Cluster IDs} \\
  \midrule
  VG-1 & CL-1, CL-3, CL-4, CL-7 \\
  %\midrule
  VG-2 & CL-1, CL-2\\
  %\midrule
  VG-3 & CL-4, CL-5, CL-6\\
  %\midrule
  VG-4 & CL-1, CL-2, CL-3, CL-4, CL-5, CL-6\\
 \bottomrule
\end{tabular}
\end{table}

The VG-VIF index aims to capture a global relationship between the VG designs and the VIF layouts to support a ranking system that allows accurate recall of the suitable VG designs given a VIF layout. To develop the VG-VIF index, we first clustered all the VIF flows in our dataset into 12 categories as mentioned in \cite{lu2020exploring}. We first generated the VIF images for each infographic in our dataset to generate these clusters. These images were then reduced to 50 dimensions using PCA \cite{joliffe1992principal} to get the principal components, which were then further reduced to 2D using t-SNE \cite{van2008visualizing}. This 2D space was divided into clusters with centers around the high-density regions with DBSCAN \cite{liu2006fast} and then iteratively clustering all the points into one of the centers. We repeated this procedure until there was no further improvement in the forming clusters. We used the same 12 classes discussed in \cite{lu2020exploring} to form the basis of the VIF layouts (denoted as CL-$X$ in Table \ref{tab:vg-vif}). 

Following this, we extracted the VG designs from each of the infographics. Table \ref{tab:vg-vif} shows an example of $4$ Visual Groups (denoted as VG-$x$) that can occur in multiple VIF flow categories (denoted as VIF-$x$). This example shows the one-to-many relationship between the VG designs and the VIF layouts. We can treat these relations as ``words'' occurring in some ``documents'', where the VGs are the documents and the corresponding cluster centers are the words in each document. 
Using this analogy, we obtain the ranking of VGs given a VIF cluster ID by calculating the \textit{TF-IDF} score \cite{ramos2003using} for each VG. The TF-IDF score has been extensively used in information retrieval and has properties that we can use to rank the VGs. Firstly, the TF-IDF score down-weights the most commonly appearing words; in this case, it results in higher rankings of less frequent VGs. Thus, our recommendation engine generates infographics using the VGs, which are less common. Also, the TF-IDF scores are generated covering the entire domain, in this case, the domain of VIFs, which is a desirable property while generating infographic designs.  

To summarize the VG ranking process, we choose the best VIF layout vectors to place the VGs based on the canvas elements. The VG scores are obtained from the VG-VIF index, which shows how well-fitting a VG is for a given layout. The VG-VIF index scores are sorted, and a subset of high-scoring VGs are selected, which match the user's markdown input (i.e., the number and type of components inside a VG). In some cases, users might want to design their own VG designs, an example of it can be a VG with some chart information. Since generating VGs with multidimensional data information is not yet supported in \name{}, users can use tools like Text-2-Viz~\cite{cui2019text} to design custom VGs and upload into \name{} to generate infographics. 
% Details of the VG-VIF ranking algorithm is discussed in the supplementary material. 
% Also, placing the VG on the VIF layout requires some fine tuning like rotation and scaling based on different user inputs and design constraints. We follow a simple process for fine tuning discussed in the supplementary material Section X. 

\subsubsection{Visual Group Placement and Information Embedding}
The ranking algorithm discussed above provides a list of VGs, which can be used with a selected VIF layout. However, placing the VG on the VIF layout requires proper rotation and scaling. The rotation of a VG is defined based on whether or not the infographic has a pivot graphic. In case the pivot graphic is present, each VG should face towards the pivot graphic, and hence the rotation angle is calculated by measuring the angle of the arc connecting the VG from the center of the pivot graphic on the circle centered at the pivot graphic. After the rotation angle for each VG is fixed, the input information can be embedded inside each VG. 

To embed the user input, each VG has placeholders defined in their respective SVG files for placing individual components (i.e., image, text, title, and label). Text's font size and dimensions of the image to be embedded are calculated based on the size of these placeholders and the content's size. Also, embedded text and images are invariant to the VG rotation and are always placed at the same angle in each of the VGs.

\section{Appendix D\\ Exceptional Cases}
Referring to the exceptional Infographic designs not covered under our framework from Section 3.1 from the paper, some examples are shown in Figure \ref{fig:fail_cases}. These cases include designs where the VGs are scaled following the VIF layout in images \textit{A}, \textit{B}, and \textit{C}. Also, in images \textit{A} and \textit{C}, the pivot graphics are composed of multiple objects and contain additional icons. Sometimes, the VG design is not fixed, as in the case of image \textit{B}. Such designs are hard to generalize with our tool, which was developed to support general-purpose infographic design and exploration. 

\begin{figure*}[tb]
    \centering
        % $\begin{array}{cccc}
    \includegraphics[width=\textwidth]{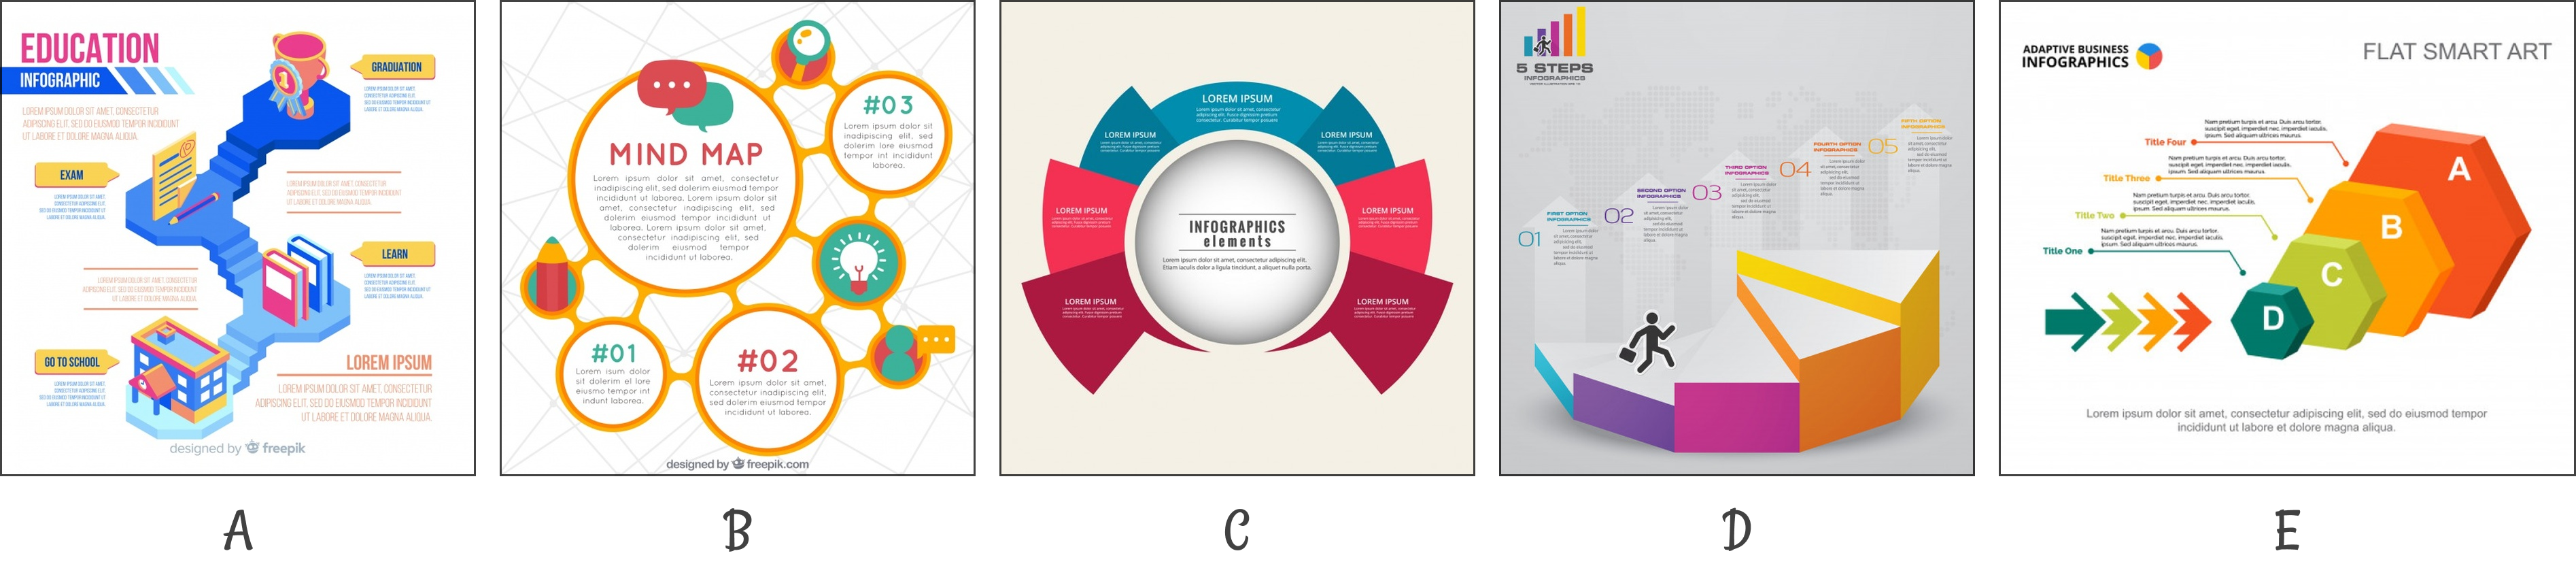}
    \caption{Infographic designs out of the scope of our framework. Some of these features include VG scaling (A, B, and C), inconsistent VG designs (A and B), complex pivot graphics composed of multiple SVG paths (A and D), and complex connection designs (E).} 
    \label{fig:fail_cases}
\end{figure*}

\section{Appendix E\\ Evaluating Design Experience with User Study}
\subsection{Tasks and Procedures}

We initially familiarized the participants with the concepts of Infographics and related terminologies, such as the definition of VG, VIF, Pivot Graphic, and Connections for our framework. Next, we showed a few examples of infographics chosen from our dataset to familiarize them with infographic designs. The participants were then allowed to experiment with \name{} and ask clarifying questions regarding the tool. 
The task was to generate an infographic design from the content and design input of choice and evaluate the design support features of \name{}. We also provided sample markdown inputs to users, and they had an option to either generate infographics from the content of their choice or use the provided examples.  
%\jian{The task is not clear. How the information is chosen. Is it prescribed or decided by the users?}

After the participants were satisfied with their generated or filtered infographic designs, we conducted a short semi-structured interview to collect qualitative feedback. 
We asked the participants to rank their experience with \name{} on a five-point Likert scale. The questionnaire was based on a total of six factors: \textit{Enjoyment}, \textit{Exploration}, \textit{Expressiveness}, \textit{Results worth the effort}, \textit{Ease of use}, and \textit{Workflow}. Four of these factors were taken from the work by Cherry \textit{et al.} \cite{cherry2014quantifying} for quantifying the creativity support for design tools. Two specific factors, \textit{Effort} and \textit{Workflow}, were added in the questionnaire to specifically evaluate \name{} for its support in infographics design and exploration tasks. 
The whole study took about 45 minutes for each participant.

% \section{Appendix F}
% \subsection{Case Studies: Demonstrating Design Capabilities with Example Cases} 
\begin{figure*}[tb]
    \centering
        % $\begin{array}{cccc}
        \includegraphics[width=\textwidth]{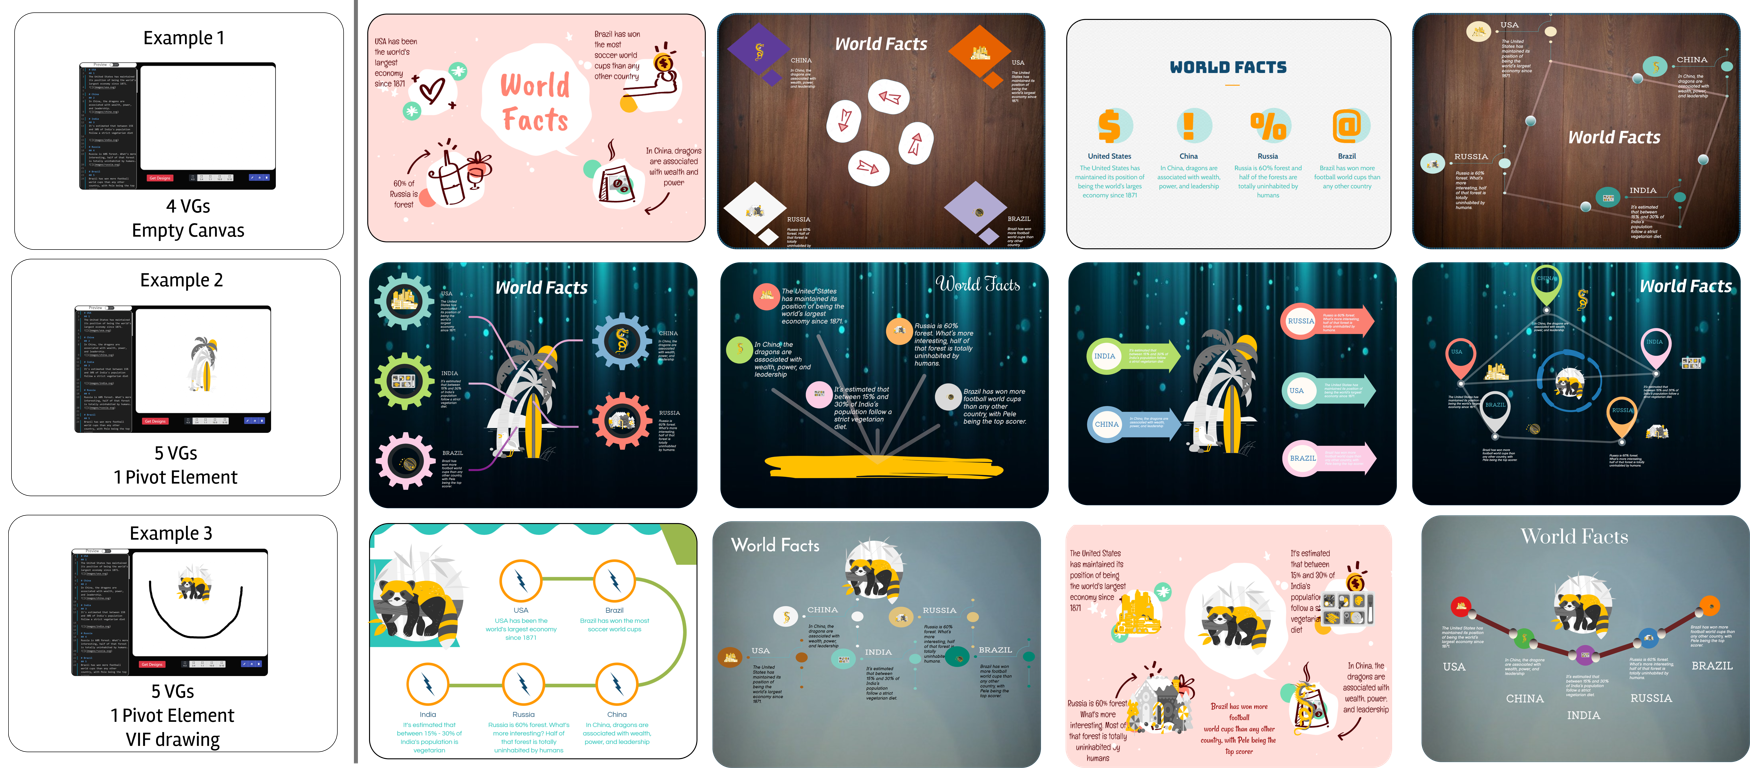}
    \caption{Example infographics generated using our framework using the example cases. We evaluated our framework with three example inputs, each of which had different content and design, shown on the left of each row. For each input, our framework recommended infographics, where we show some recommended infographics in each row for similar inputs.} 
    \label{fig:example_cases}
\end{figure*}

\begin{figure*}[tb]
 \centering
 \includegraphics[width=\textwidth]{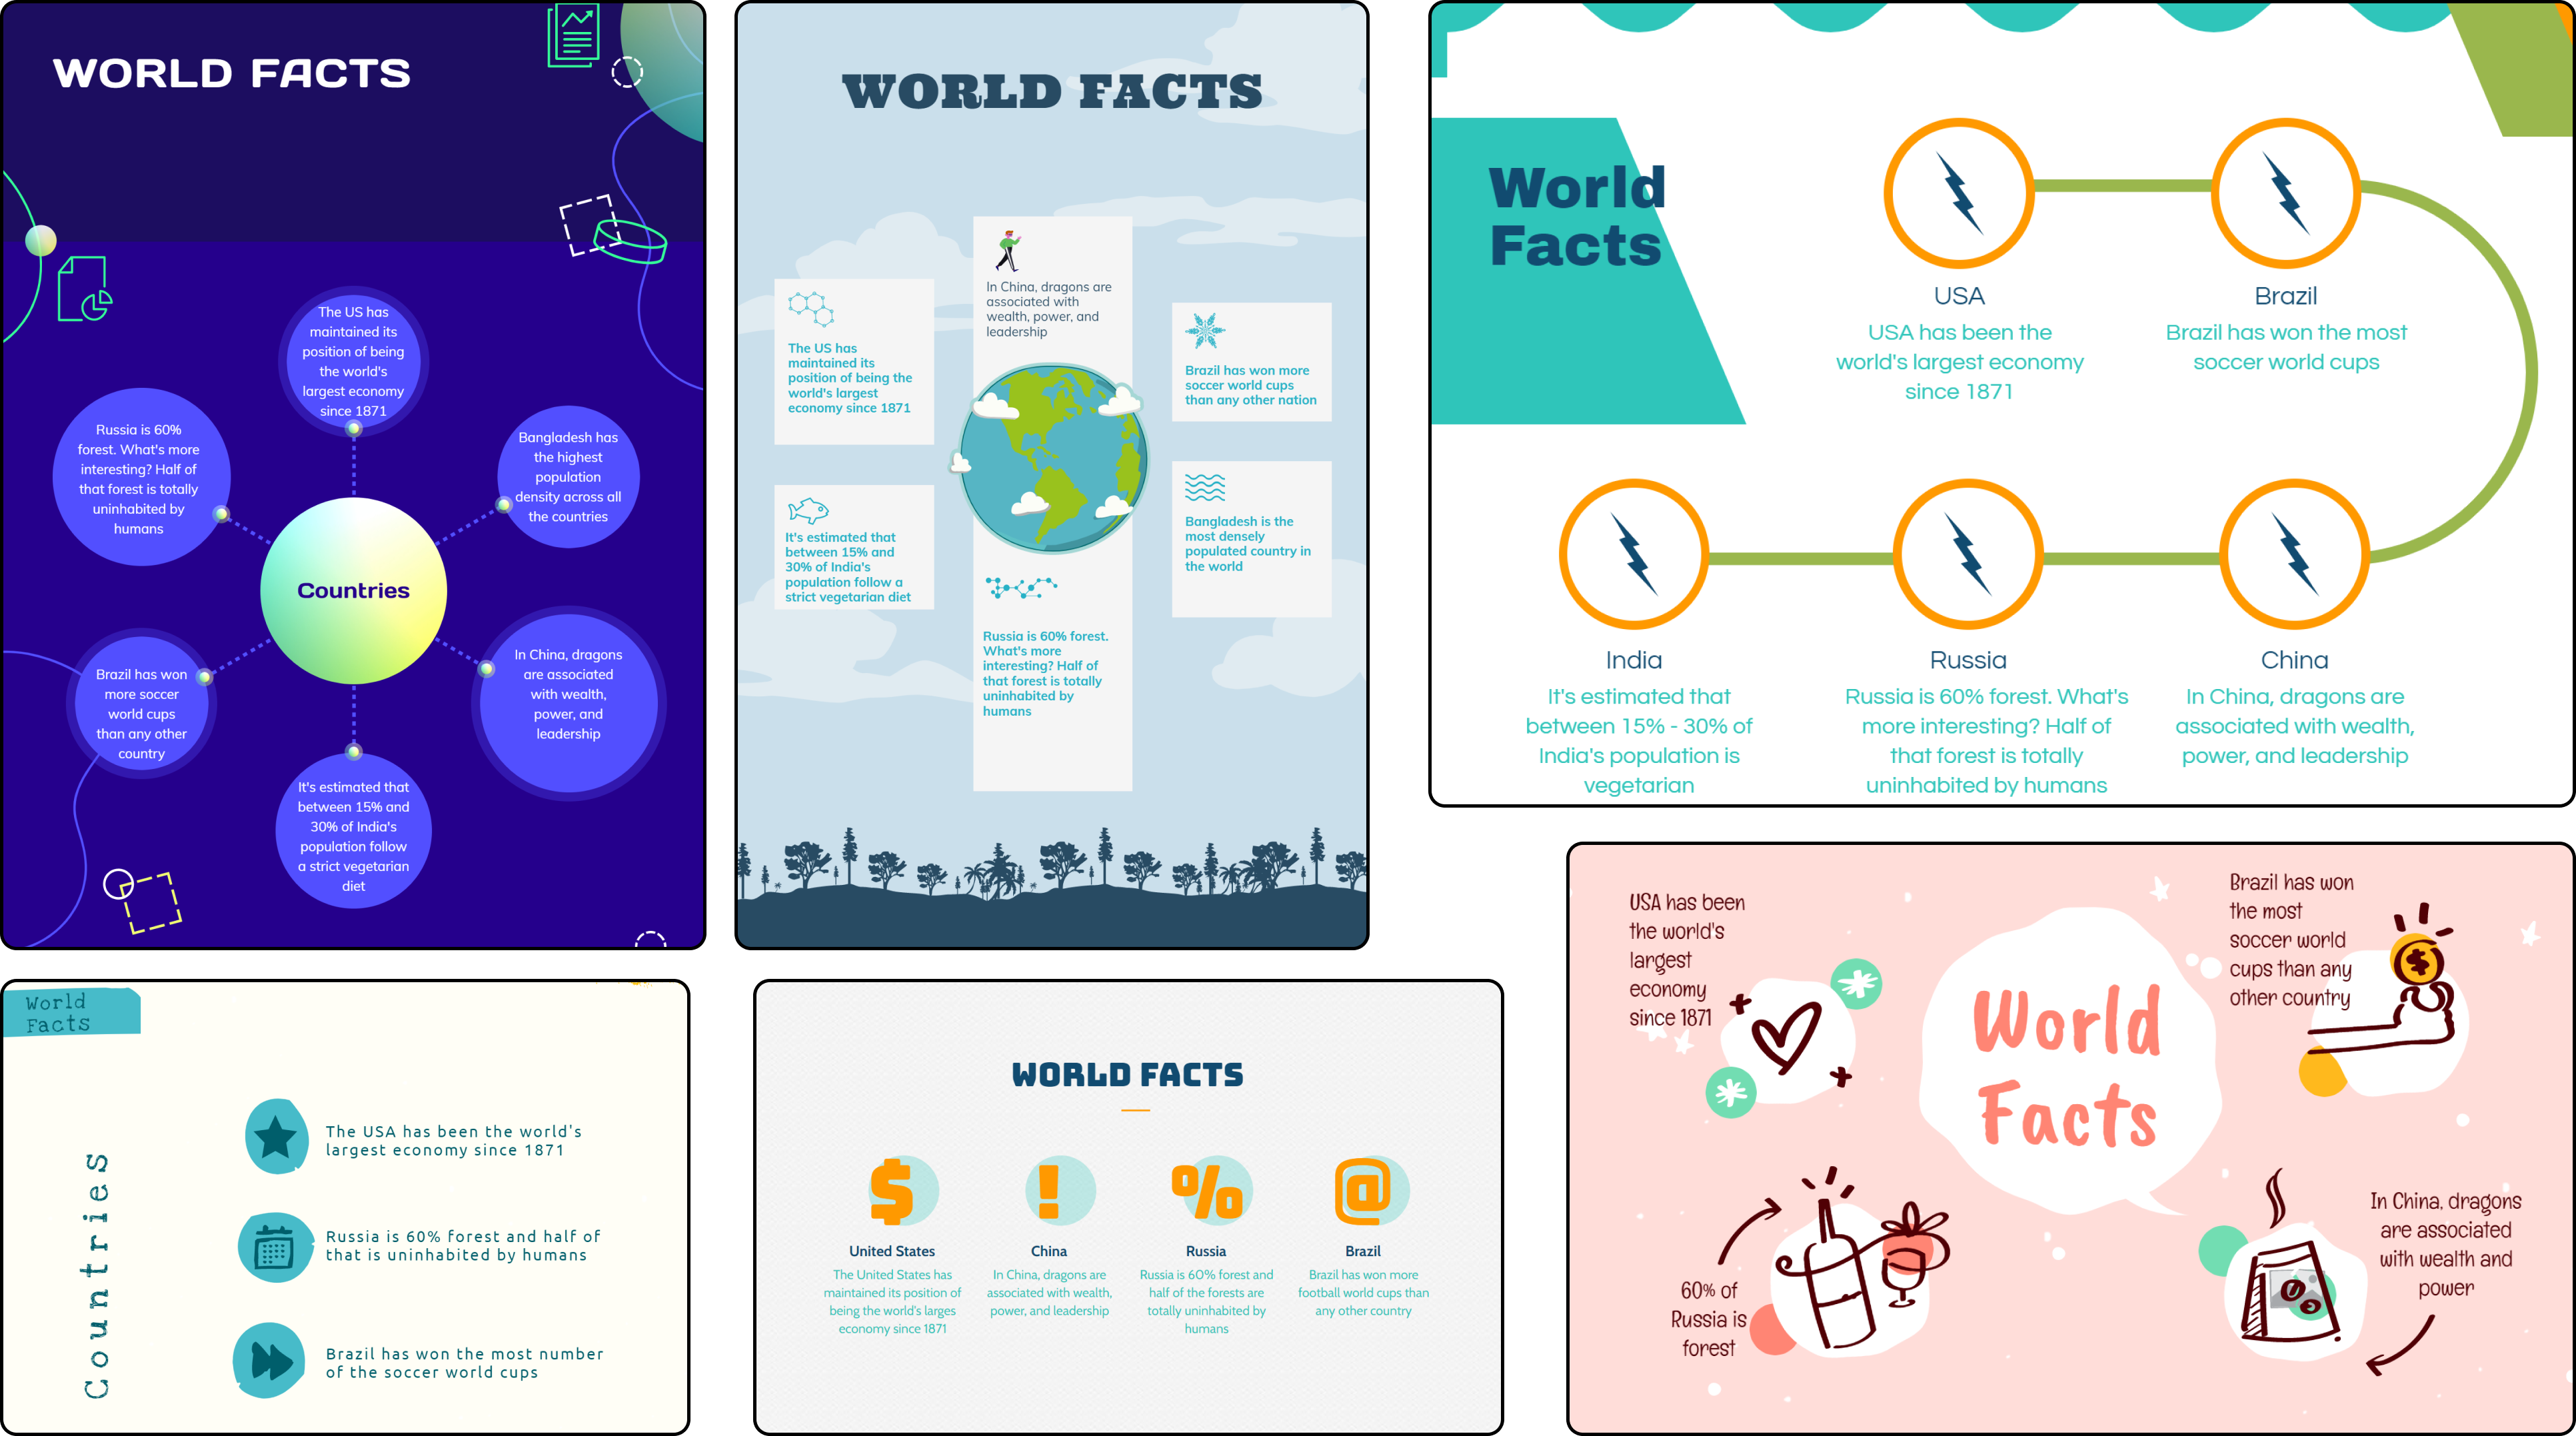}
 \vspace{-6mm}
 \caption{Sample infographic designs generated with our framework collected during a user study. 
%  Images and text in the infographics are user inputs while the overall designs are generated using our framework. More results are provided in the supplementary materials. 
}
 \label{fig:collage}
\end{figure*}

% Also, our tool generates designs by perfectly placing the markdown content inside varying VG designs with proper scaling and wrapping for all the example inputs. Using \name{}, the designer can optionally change the background of the canvas, connection designs, and types, and VG color pallets using the menu bar on \name{} (Figure \ref{fig:teaser}). Following up on the results from all the example inputs, we can conclude that our framework is able to generate infographic designs for varying design scenarios. 

% Figure \ref{fig:example_cases} shows the generated recommendations with three different pivot elements for Example 2, where \name{} is able to generate infographic designs based on the shape of the pivot element. 

 %while still providing designers with the option to control the design with necessary feedback.
